# Supplementary material for: Performance Analysis of 6G Multiuser Massive MIMO-OFDM THz Wireless Systems with Hybrid Beamforming under Intercarrier Interference
Source: arXiv:2401.12351 source file (2024-01-22)
Supplement: Supplementary file 1 [file app0A.tex]

%
% file: localoperator.tex
% author: Victor Brena
% description: Briefly describes properties of the local operator.
%

\chapter{Appendix A}
\label{app:app01}

An appendix

\
